# Supplementary material for: RoomDiffusion: A Specialized Diffusion Model in the Interior Design Industry
Source: arXiv:2409.03198 source file (2024-09-05)
Supplement: Supplementary file 1 [file appendix.tex]

\newpage
\appendix
\section{Appendix}
\subsection{Public Datasets Details}
\begin{table*}[hp!]
    \centering
    \caption{Complete Overview of two public MICCAI Chanllenge Datasets}
    \begin{adjustbox}{width=\textwidth}
    \begin{tabular}{*{1}{l}|*{3}{c}}
        % \hline \hline
        \toprule
        MICCAI Challenge & AMOS2022 & FLARE2021 \\
        \midrule
        Imaging Modality & Multi-Contrast CT & Multi-Contrast CT \\
        Anatomical Region & Abdomen & Abdomen \\
        Dimensions & ${512-768}\times{512-768}\times\{68-353$\} & $512\times512\times\{37-751$\} \\
        Resolution & $\{0.45-1.07\}\times\{0.45-1.07\}\times\{1.25-5.00\}$ & $\{0.61-0.98\}\times\{0.61-0.98\}\times\{0.50-7.50\}$ \\
        Sample Size & 200 & 361 \\
        \midrule
        \multirow{3}{*}{Anatomical Label} & Spleen, Left \& Right Kidney, Gall Bladder, \\
        & Esophagus, Liver, Stomach, Aorta, Inferior Vena Cava (IVC), 
        & Spleen, Kidney \\
        & Pancreas, Left \& Right Adrenal Gland (AG), Duodenum, 
        & Liver, Pancreas \\
        & Bladder, Prostates/uterus \\
        \midrule
        \multirow{2}{*}{Data Splits} & 5-Fold Cross-Validation & 5-Fold Cross-Validation\\
        & Train: 160 / Validation: 20 / Test: 20 & Train: 289 / Validation: 36 / Test: 36  \\
        \bottomrule
    \end{tabular}
    \end{adjustbox}
    \label{baselines_compare}
\end{table*}

\subsection{Data Preprocessing \& Model Training}

We apply a series of hierarchical steps for data preprocessing:
\begin{enumerate}
\item[1).] The provided training cases are cropped to their nonzero region.
\item[2).] Intensity clipping is applied to further enhance the contrast of soft tissue (AMOS2022:\{min:-992, max:374\} \& FLARE2021:\{min:-16, max:270\}).
\item[3).] Resample all training cases to a unified spacing(AMOS2022:[2, 0.6846, 0.6846] \& FLARE2021:[1, 0.8164, 0.8164]).
\item[4).] Apply image normalization processing(AMOS2022:\{mean:47.3369, sd:145.1008\} \& FLARE2021:\{mean:116.6280, sd:47.8994\}).
\end{enumerate}
Details regarding training parameters and data augmentation are summarized in Table\ref{aug}.

\newpage
\subsection{Pre-training Datasets}
This section describes the details of pre-training. The proposed Springboard-UNETR is pre-trained on five different datasets, and the information for these datasets is shown in the table~\ref{pretrain dataset}. Similar to SwinUNETR, we have conducted a variety of self-supervised training methods on the encoder component of the model, including reconstruction, rotation, and comparison. The entire training process adopts an input size of [128, 128, 128] and trains continuously for 100000 steps.

\begin{table*}[hp!]
    \centering
    \caption{Hyperparameters of both directly training and finetuning scenarios on three public datasets}
    \begin{adjustbox}{width=0.5\textwidth}
    \begin{tabular}{*{1}{l}|*{2}{c}}
        % \hline \hline
        \toprule
        \textbf{Hyperparameters} & \textbf{Training} \\
        \midrule
        Training Epoch & 1000 \\
        Batch Size & 2  \\
        Optimizer & SGD \\
        Momentum & 0.99 \\
        Learning Rate & $1e-2$ \\
        Weight Decay & $3e-5$ \\
        Patch Size & (128, 128, 128) \\
        \midrule
        \textbf{Data Augmentation} &  \textbf{Value} \\
        \midrule
        Elastic Deform Coordinates & \checkmark \\
        Elastic Alpha & (0, 900) \\
        Elastic Sigma & (9, 13) \\
        Scale Range & (0.85, 1.25) \\
        Gamma Range & (0.7, 1.5) \\
        Mirror Axes & x, y, z \\
        Rotation Degree & $-30^{\circ}$ to $+30^{\circ}$ \\
        Oversample Foreground & \checkmark \\
        Oversample Foreground Percent & 0.33 \\
         \bottomrule
    \end{tabular}
    \end{adjustbox}
    \label{aug}
\end{table*}

\begin{table*}[hp!]
    \centering
    \caption{Summary of datasets for pre-training, the use of cohorts identifies diversified regions of interest}
    \begin{adjustbox}{width=1\textwidth}
    \begin{tabular}{*{1}{l}|*{5}{c}} 
        % \hline \hline
        \toprule
        Dataset   &Region of Interest & \#Total Samples & Source & Train/Validation \\ 
        \midrule
        MSD & Abdomen   & 420  & https://decathlon-10.grand-challenge.org  & 350/70 \\ 
        KITS & Abdomen & 370  & https://github.com/neheller/kits19 & 300/70 \\
        LITS & Abdomen & 201 & https://competitions.codalab.org/competitions/17094#learn_the_details & 130/71 \\
        BTCV & Abdomen & 50 & https://www.synapse.org/#!Synapse:syn3193805/wiki/89480 & 30/20\\
        LiDC & Chest & 475 & https://wiki.cancerimagingarchive.net/pages/viewpage.action?pageId=1966254 & 451/24 \\
         \bottomrule
    \end{tabular}
    \end{adjustbox}
    \label{pretrain dataset}
\end{table*}
